# Supplementary material for: Understanding Reasoning in Chain-of-Thought from the Hopfieldian View
Source: arXiv:2410.03595 source file (2024-10-04)
Supplement: Supplementary file 2 [file appendix-aqua-prompt.tex]

\begingroup
\begin{table*}[!ht]
    \centering
    \small
    \begin{tabular}{p{0.8\linewidth}}
        \toprule
        \underline{\textbf{\textsc{Prompt for AQuA algebraic word problems}}} \\
        \vspace{-2mm}
        \textbf{Q:} John found that the average of 15 numbers is 40. If 10 is added to each number then the mean of the numbers is? \\ Answer Choices: (a) 50 (b) 45 (c) 65 (d) 78 (e) 64 \\
        \vspace{-1mm}
        \textbf{A:} \hl{If 10 is added to each number, then the mean of the numbers also increases by 10. So the new mean would be 50.} The answer is (a). \\
         \vspace{0mm}
        \textbf{Q:} If a / b = 3/4 and 8a + 5b = 22,then find the value of a. \\ Answer Choices: (a) 1/2 (b) 3/2 (c) 5/2 (d) 4/2 (e) 7/2 \\
        \vspace{-1mm}
        \textbf{A:} \hl{If a / b = 3/4, then b = 4a / 3. So 8a + 5(4a / 3) = 22. This simplifies to 8a + 20a / 3 = 22, which means 44a / 3 = 22. So a is equal to 3/2.} The answer is (b). \\
        \vspace{0mm}
        \textbf{Q:} A person is traveling at 20 km/hr and reached his destiny in 2.5 hr then find the distance? \\ Answer Choices: (a) 53 km (b) 55 km (c) 52 km (d) 60 km (e) 50 km \\
        \vspace{-1mm}
        \textbf{A:} \hl{The distance that the person traveled would have been 20 km/hr * 2.5 hrs = 50 km.}  The answer is (e). \\
        \vspace{0mm}
        \textbf{Q:} How many keystrokes are needed to type the numbers from 1 to 500? \\ Answer Choices: (a) 1156 (b) 1392 (c) 1480 (d) 1562 (e) 1788 \\
        \vspace{-1mm}
        \textbf{A:} \hl{There are 9 one-digit numbers from 1 to 9. There are 90 two-digit numbers from 10 to 99. There are 401 three-digit numbers from 100 to 500. 9 + 90(2) + 401(3) = 1392.} The answer is (b). \\
        \bottomrule
    \end{tabular}
    \caption{
    Few-shot exemplars for full chain of thought prompt for AQuA.
    }
    \label{tab:appendix-aqua-prompt}
\end{table*}
\endgroup
