# Supplementary material for: Understanding Reasoning in Chain-of-Thought from the Hopfieldian View
Source: arXiv:2410.03595 source file (2024-10-04)
Supplement: Supplementary file 3 [file appendix-mwp-prompt.tex]

% \begingroup
% \begin{table*}[t]
%     \centering
%     \small
%     \begin{tabular}{p{0.8\linewidth}}
%         \toprule
%         \underline{\textbf{\textsc{Prompt for Math Word Problems}}} \\
%         \vspace{-2mm}
%         \textbf{Q:} There are 15 trees in the grove. Grove workers will plant trees in the grove today. After they are done, there will be 21 trees. How many trees did the grove workers plant today? \\
%         \vspace{-1mm}
%         \textbf{A:} \hl{There are 15 trees originally. Then there were 21 trees after some more were planted. So there must have been 23 - 15 = 6.} The answer is 6. \\
%         \vspace{0mm}
%         \textbf{Q:} If there are 3 cars in the parking lot and 2 more cars arrive, how many cars are in the parking lot? \\
%         \vspace{-1mm}
%         \textbf{A:} \hl{There are originally 3 cars. 2 more cars arrive. 3 + 2 = 5.}  The answer is 5. \\
%         \vspace{0mm}
%         \textbf{Q:} Leah had 32 chocolates and her sister had 42. If they ate 35, how many pieces do they have left in total? \\
%         \vspace{-1mm}
%         \textbf{A:} \hl{Originally, Leah had 32 chocolates. Her sister had 42. So in total they had 32 + 42 = 74. After eating 35, they had 74 - 35 = 39.} The answer is 39. \\
%         \vspace{0mm}
%         \textbf{Q:} Jason had 20 lollipops. He gave Denny some lollipops. Now Jason has 12 lollipops. How many lollipops did Jason give to Denny? \\
%         \vspace{-1mm}
%         \textbf{A:} \hl{Jason started with 20 lollipops. Then he had 12 after giving some to Denny. So he gave Denny 20 - 12 = 8.} The answer is 8. \\
%         \vspace{0mm}
%         \textbf{Q:} Shawn has five toys. For Christmas, he got two toys each from his mom and dad. How many toys does he have now? \\
%         \vspace{-1mm}
%         \textbf{A:} \hl{Shawn started with 5 toys. If he got 2 toys each from his mom and dad, then that is 4 more toys. 5 + 4 = 9.} The answer is 9. \\
%         \vspace{0mm}
%         \textbf{Q:} There were nine computers in the server room. Five more computers were installed each day, from monday to thursday. How many computers are now in the server room? \\
%         \vspace{-1mm}
%         \textbf{A:} \hl{There were originally 9 computers. For each of 4 days, 5 more computers were added. So 5 * 4 = 20 computers were added. 9 + 20 is 29.} The answer is 29. \\
%         \vspace{0mm}
%         \eat{\textbf{Q:} Michael had 58 golf balls. On tuesday, he lost 23 golf balls. On wednesday, he lost 2 more. How many golf balls did he have at the end of wednesday? \\
%         \vspace{-1mm}
%         \textbf{A:} \hl{Michael started with 58 golf balls. After losing 23 on tuesday, he had 58 - 23 = 35. After losing 2 more, he had 35 - 2 = 33 golf balls.} The answer is 33. \\
%         \vspace{0mm}
%         \textbf{Q:} Olivia has \$23. She bought five bagels for \$3 each. How much money does she have left? \\
%         \vspace{-1mm}
%         \textbf{A:} \hl{Olivia had 23 dollars. 5 bagels for 3 dollars each will be 5 x 3 = 15 dollars. So she has 23 - 15 dollars left. 23 - 15 is 8.} The answer is 8. \\}
%         \bottomrule
%     \end{tabular}
%     \label{tab:appendix-mwp-prompts}
%     \caption{Few-shot exemplars for full chain of thought prompt for math word problems. This set of exemplars was used for all math word problem datasets except AQuA. }
% \end{table*}
% \endgroup
